# Supplementary material for: Charge disproportionation driven polar magnetic metallic double-layered perovskite Sr$_3$Co$_2$O$_7$
Source: arXiv:2511.01749 source file (2025-11-03)
Supplement: Supplementary file 1 [file sm.pdf]

# Supplementary Materials: Charge disproportionation driven polar magnetic metallic double-layered perovskite $Sr_3Co_2O_7$

Hong-Fei Huang,[1] Houssam Sabri,[2] Jiadong Zang,[2] and Jie-Xiang Yu[1]

[1]*School of Physical Science and Technology, Soochow University, Suzhou 215006, China*
[2]*Department of Physics and Astronomy, University of New Hampshire, Durham, New Hampshire 03824, USA*

## I. TOTAL ENERGY RESULTS FOR $U$ PARAMETERS

Table S1. Relative total energies for states with centrosymmetric/asymmetric (SYM/FE) and ferromagnetic/A-type antiferromagnetic (FM/A-AF) phases under different $U$ parameters (units: eV) for $+U$ method. All results use $J = 0.9$ eV.

| $E$(meV per Co) | $U = 4.0$ | $U = 5.0$ | $U = 6.0$ |
|---|---|---|---|
| SYM+FM | 0.0 | 0.0 | 0.0 |
| SYM+A-AF | 80.6 | 3.8 | 5.6 |
| FE+FM | -35.0 | -84.0 | -33.5 |
| FE+A-AF | -21.5 | -72.0 | -21.0 |

## II. ELASTIC ENERGY OF THE FE PHASE

Both the SYM and FE phases are dynamically stable without soft modes. In the SYM phase, the apical Oz atom occupies an inversion center, rendering Co1 and Co2 symmetry equivalent. The Co1-Oz-Co2 bond is symmetrically balanced along $z$-direction, where both the Co-O bond length is 1.88 Å. Relative to the equilibrium SYM phase, Co1 is displaced upward by 0.08 Å with respect to Co2, while Oz atom is displaced downward by 0.08 Å. Consequently, the bond lengths change from their equilibrium to 2.04 and 1.80 Å, respectively, generating a total strain of approximately 0.24 Å.

It is clear that the displacement of Oz introduces an additional elastic energy via the induced strain. To quantify the energy change further, we approximate the response using Hooke's law, which gives the elastic energy as $E_{el} = 1/2kx^2$. Here, $k$ is the force constant and $x$ is the total elastic strain. We next impose finite displacements on the Oz atom of the SYM phase and extract an effective force constant by fitting the resulting total-energy variations. When it deviates from the center position by 0.01 Å, the total strain generated is 0.02 Å, and at this point, the total energy increases by 0.41 meV. Neglecting the minor charge effects, we thereby obtain $k \approx 2.07$ eV/Å for the out-of-plane Co–O bonds in this case. Ultimately, the elastic energy contribution from the ferroelectric displacement is +29.9 meV (or 15 meV per Co), where the positive sign indicates an increase in total energy.

## III. ELECTRONIC ENERGY BY CHARGE DISPROPORTIONATION

Start from Eq. (9) of Anisimov's work [Ref. 10.1103/PhysRevB.44.943 in the main text], the single particle potential of Hubbard $U$ for each orbital with orbital index $m$ and spin index $\sigma$ is given by:

$$V_{m\sigma}^{(U)} = U \sum_{m'} (n_{m'-\sigma} - n_0) + (U - J) \sum_{m' \neq m} (n_{m'\sigma} - n_0) \tag{S1}$$

$$= U \sum_{m'} n_{m'-\sigma} + (U - J) \sum_{m' \neq m} n_{m'\sigma} - \frac{9}{10} U n_d + \frac{4}{10} J n_d \tag{S2}$$

$$= U (n_d - n_{m\sigma}) - J (n_\sigma - n_{m\sigma}) - \frac{9}{10} U n_d + \frac{4}{10} J n_d \tag{S3}$$

$$= U n_d - J n_\sigma - (U - J) n_{m\sigma} - \frac{9}{10} U n_d + \frac{4}{10} J n_d \tag{S4}$$

$$= -J n_\sigma - (U - J) n_{m\sigma} + \frac{1}{10} (U + 4J) n_d \tag{S5}$$

where $n_0 = n_d/10$, $n_d = n_\sigma + n_{-\sigma} = n_\uparrow + n_\downarrow = \sum_{m,\sigma} n_{m\sigma}$, and $n_\sigma = \sum_m n_{m\sigma}$.

In $Sr_3Co_2O_7$, $U = 4.0$ eV and $J = 0.9$ eV is used. The corresponding occupancies of Co for SYM and FE phase are listed in Table S2.

Table S2. The corresponding occupancies, the potential correction for the corresponding $t_{2g}$ orbitals, $\Delta V = V_{(xz/yz)\downarrow} - V_{xy\downarrow}$ and the total energy correction correction by $U$ of each Co for SYM and FE phase in FM ordering.

| | $n_\uparrow$ | $n_\downarrow$ | $n_d$ | $n_{(xz/yz)\downarrow}$ | $n_{xy\downarrow}$ | $V_{(xz/yz)\downarrow}$ (eV) | $V_{xy\downarrow}$ (eV) | $\Delta V$ (eV) | $E^{(U)}$ (eV) |
|---|---|---|---|---|---|---|---|---|---|
| Co in SYM+FM | 4.33 | 2.62 | 6.95 | 0.50 | 1.00 | 1.37 | -0.18 | 1.55 | 0.511 |
| Co1 in FE+FM | 4.16 | 2.85 | 7.01 | 0.98 | 0.32 | -0.28 | 1.77 | -2.05 | 0.297 |
| Co2 in FE+FM | 4.41 | 2.46 | 6.87 | 0.38 | 1.00 | 1.83 | -0.09 | 1.92 | 0.602 |

Then we can have the potential correction by Hubbard $U$ and the corresponding single particle energy correction as $E_{m\sigma}^{(U)} = n_{n\sigma} V_{m\sigma}^{(U)}$ for each orbital. The total energy correction for each Co is $E^{(U)} = \sum_{m\sigma} E_{m\sigma}^{(U)}$. They are also listed in Table S2. $\Delta V$ corresponds to the additional crystal field splitting caused by occupancies and Hubbard $U$ of $d$ orbitals, so that the magnitude of crystal field splitting between $d_{(xz/yz)\downarrow}$ and $d_{xy\downarrow}$ for FE phase is larger than SYM. As a result, FE have 0.123 eV per two Co (or 61 meV per Co) lower in Hubbard $U$ energy than SYM phase.

## IV. EXCHANGE ANALYSIS FOR CO1-CO2

We focus on the model along the exchange pathway of Co1-Oz-Co2 containing the Co($t_{2g}$) and Oz($p$) orbitals of the FE phase. There are two exchange pathways via $pd\pi$ bonding: Co1($d_{xz}$)-Oz($p_x$)-Co2($d_{xz}$) and Co1($d_{yz}$)-Oz($p_y$)-Co2($d_{yz}$). $d_{xy}$ is not involved. In both the ferromagnetic (FM) and A-type antiferromagnetic (A-AF) cases, the two pathways are degenerate. For simplicity, only one pathway will be discussed and $d_1$, $d_2$ and $p$ is used to denote the corresponding orbitals of Co1, Co2 and Oz respectively in the following.

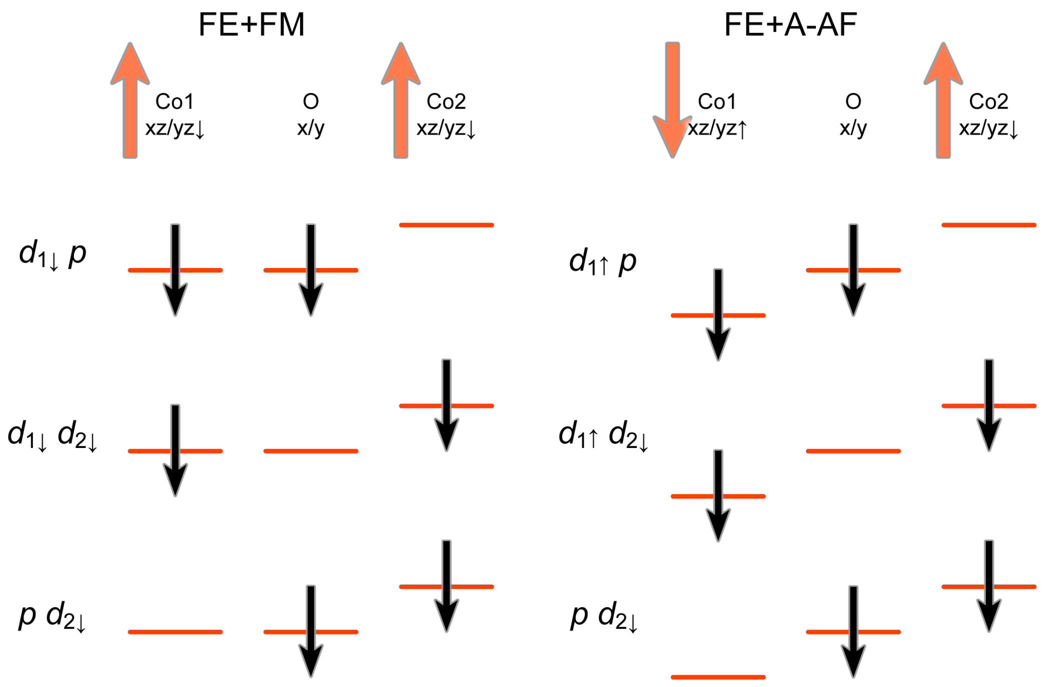


Figure S1. The diagram for the single electron states considered in the exchange models for FM and A-AF phase respectively.

when Co1 and Co2 have the FM coupling, the spin up channel is the spin majority for both Co1 and Co2. All $t_{2g}$ and $p$ orbitals are occupied in the spin majority channel with no exchange energy. In the spin minority channel, the single electron ground state is that Co1($d_{xz}/d_{yz}$), Co2($d_{xy}$) and Oz($p_{x/y}$) is occupied. Since $d_{xy}$ is not involved in the exchange along $d_1 - p - d_2$, the state is labeled as $(d_{1\downarrow}p)$ with two electrons occupied. The on-site energy for $(d_{1\downarrow}p)$ is $\varepsilon_1 + \varepsilon_p + U'$ where $\varepsilon_1$ and $\varepsilon_p$ is the orbital energy of Co1($d_{xz}/d_{yz}$) and Oz($p_x/p_y$) respectively and $U'$ is the effective on-site Coulomb interaction energy for cobalt. Other exciting states are $(d_{1\downarrow}d_{2\downarrow})$ and $(pd_{2\downarrow})$, shown in Fig.S1 with the on-site energy $\varepsilon_1 + \varepsilon_2 + 2U'$ and $\varepsilon_2 + \varepsilon_p + U'$ respectively. The hopping parameters of $(d_{1\downarrow}p) - (d_{1\downarrow}d_{2\downarrow})$ and $(d_{1\downarrow}d_{2\downarrow}) - (pd_{2\downarrow})$ are $t_1$ and $t_2$ respectively. Now the many body effective Hamiltonian under the single electron picture is given by:

$$\mathcal{H}_{\text{FM}} = \begin{matrix} \langle d_{1\downarrow}p| \\ \langle d_{1\downarrow}d_{2\downarrow}| \\ \langle pd_{2\downarrow}| \end{matrix} \begin{pmatrix} 0 & t_1 & \\ t_1 & \varepsilon_2 - \varepsilon_p + U' & t_2 \\ & t_2 & \varepsilon_2 - \varepsilon_1 \end{pmatrix} \tag{S6}$$

where the on-site energy for $(d_{1\downarrow}p)$ is set to zero.

Since $U'$ is much larger than $|t_1|$ and $|t_2|$, we need to calculate the energy correction of the ground state $(d_{1\downarrow}p)$ under perturbation theory. The second order perturbation correction is $\Delta^{(2)}_{\text{FM}} = -\frac{t_1^2}{\varepsilon_2 - \varepsilon_p + U'} < 0$ which is trivial for superexchange. The energy

correction of $(d_{1\downarrow}d_{2\downarrow})$ by $(pd_{2\downarrow})_{\downarrow}$ is $\delta = \frac{t_2^2}{U'+\varepsilon_1-\varepsilon_p} > 0$. So the fourth order perturbation correction is

$$\begin{aligned}\Delta^{(4)}_{\mathrm{FM}} &\approx -\frac{1}{\varepsilon_2 - \varepsilon_p + U'}\Delta^{(2)}\delta \\ &\approx \frac{t_1^2 t_2^2}{\left(\varepsilon_1 - \varepsilon_p + U'\right)\left(\varepsilon_2 - \varepsilon_p + U'\right)^2} > 0\end{aligned} \tag{S7}$$

Under the A-AF case, the spin-up channel is the spin minority for Co1 and spin majority for Co2, and the spin-down channel involves the spin majority for Co1 and spin minority for Co2. Since Co1$(d_{xz}/d_{yz})$ is occupied in the spin minority, all orbitals involved in the pathway along $d_1 - p - d_2$ in spin-up channel is occupied, so that no exchange energy emerges from this spin channel. In the spin-down channel, Co2$(d_{xz}/d_{yz})$ is unoccupied in the spin minority, so that this pathway can reduce the ground state energy. Here we label the occupancy of Co1$(d_{xz}/d_{yz})$ in the spin majority as $(d_{1\uparrow})$ and the corresponding orbital energy is $\varepsilon_1'$. The corresponding states are shown in Fig.S1. Now we can write the effective Hamiltonian for A-AF ordering as:

$$\mathcal{H}_{\text{A-AF}} = \begin{matrix} \langle d_{1\uparrow}p| \\ \langle d_{1\uparrow}d_{2\downarrow}| \\ \langle pd_{2\downarrow}| \end{matrix} \begin{pmatrix} 0 & t_1 & \\ t_1 & \varepsilon_2 - \varepsilon_p + U' & t_2 \\ & t_2 & \varepsilon_2 - \varepsilon_1' \end{pmatrix} \tag{S8}$$

where the energy of the single electron ground state $(d_{1\uparrow}p)$ is also set to zero.

The second order perturbation correction for $(d_{1\uparrow}p)$ is $\Delta^{(2)}_{\text{A-AF}} = -\frac{t_1^2}{\varepsilon_2-\varepsilon_p+U'}$ which is the same for the FM case. The fourth order correction is

$$\Delta^{(4)}_{\text{A-AF}} \approx \frac{t_1^2 t_2^2}{\left(\varepsilon_1' - \varepsilon_p + U'\right)\left(\varepsilon_2 - \varepsilon_p + U'\right)^2} \tag{S9}$$

where the only difference with $\Delta^{(4)}_{\mathrm{FM}}$ is the orbital energy $\varepsilon_1'$. $\varepsilon_1' < \varepsilon_1$ because of the spin splitting and the fourth order correction is positive, so that we get $\Delta^{(4)}_{\mathrm{FM}} < \Delta^{(4)}_{\text{A-AF}}$. The FM phase has the lower energy than the A-AF phase. The energy difference between FM and A-AF ordering can be estimated as

$$\begin{aligned} E_{\text{A-AF}} - E_{\mathrm{FM}} &= \Delta^{(4)}_{\text{A-AF}} - \Delta^{(4)}_{\mathrm{FM}} \\ &= \frac{t_1^2 t_2^2}{\left(\varepsilon_2 - \varepsilon_p + U'\right)^2}\left[\frac{1}{\left(\varepsilon_1' - \varepsilon_p + U'\right)} - \frac{1}{\left(\varepsilon_1 - \varepsilon_p + U'\right)}\right] \\ &\approx \frac{t_1^2 t_2^2}{U'^4}(\varepsilon_1 - \varepsilon_1') \end{aligned} \tag{S10}$$

where the approximation $U' \gg |\varepsilon_1 - \varepsilon_p|, |\varepsilon_1' - \varepsilon_p|, |\varepsilon_2 - \varepsilon_p|$ is applied in the last step. Because of the degenerate exchange pathways of Co1$(d_{xz})$-Oz$(p_x)$-Co2$(d_{xz})$ and Co1$(d_{yz})$-Oz$(p_y)$-Co2$(d_{yz})$, the actual energy difference should be doubled.

Based on the Wannier function-based Hamiltonian, $|t_1| = 0.6\,\mathrm{eV}$ and $|t_2| = 1.0\,\mathrm{eV}$ for both the FM and A-AF state. The effective on-site Coulomb interaction $U' \sim 3 - 4\,\mathrm{eV}$ for cobalt cations and $\varepsilon_1 - \varepsilon_1'$, the spin splitting energy for $d_{xz}/d_{yz}$, is about $1.0\,\mathrm{eV}$. Then we can eventually estimate the energy difference between the FM and A-AF state is about $4 - 9\,\mathrm{meV}$, qualitatively consistent with the total energy results from the first-principles calculations.

## V. ELECTRONIC STRUCTURES OF THE FE PHASE IN A $2 \times 2 \times 1$ SUPERCELL WITH ONE OXYGEN VACANCY

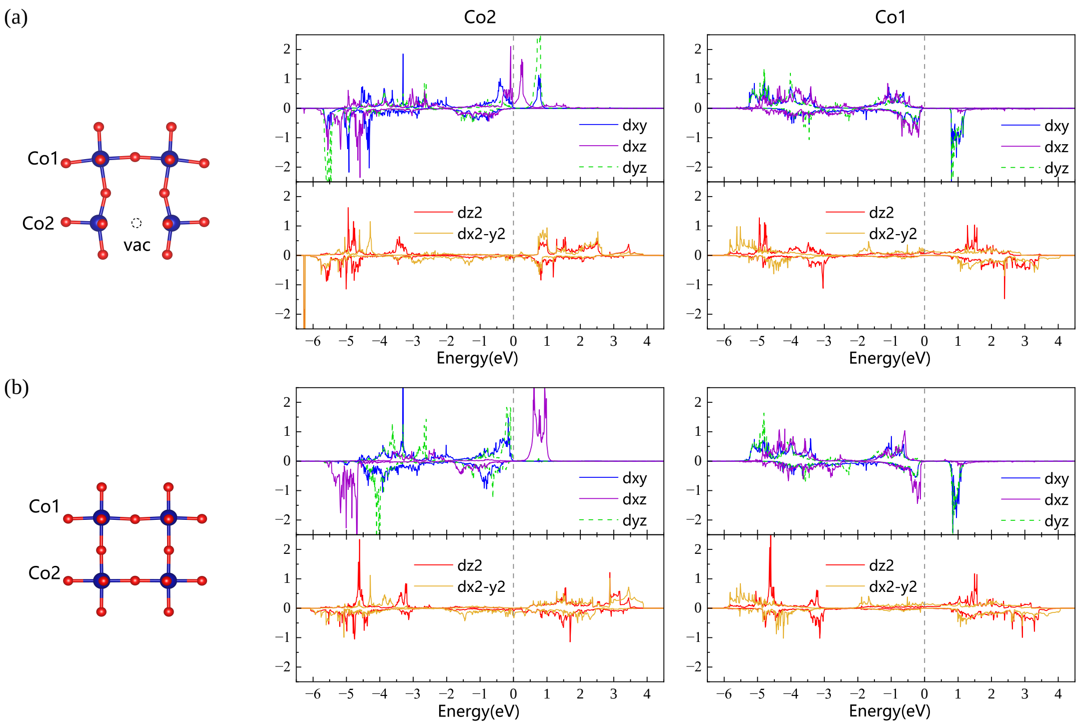


Figure S2. The projected density of states (PDOS) of Co($3d$) orbitals in the FE phase supercell with an oxygen vaccancy at the planar O2xy site. (a) The two Co atoms adjacent along the $z$-direction near the O vaccancy, where Co2 missing one Co-O bond and Co1 retaining finite electric dipole. (b) The two Co atoms located diagonally opposite the vacancy.

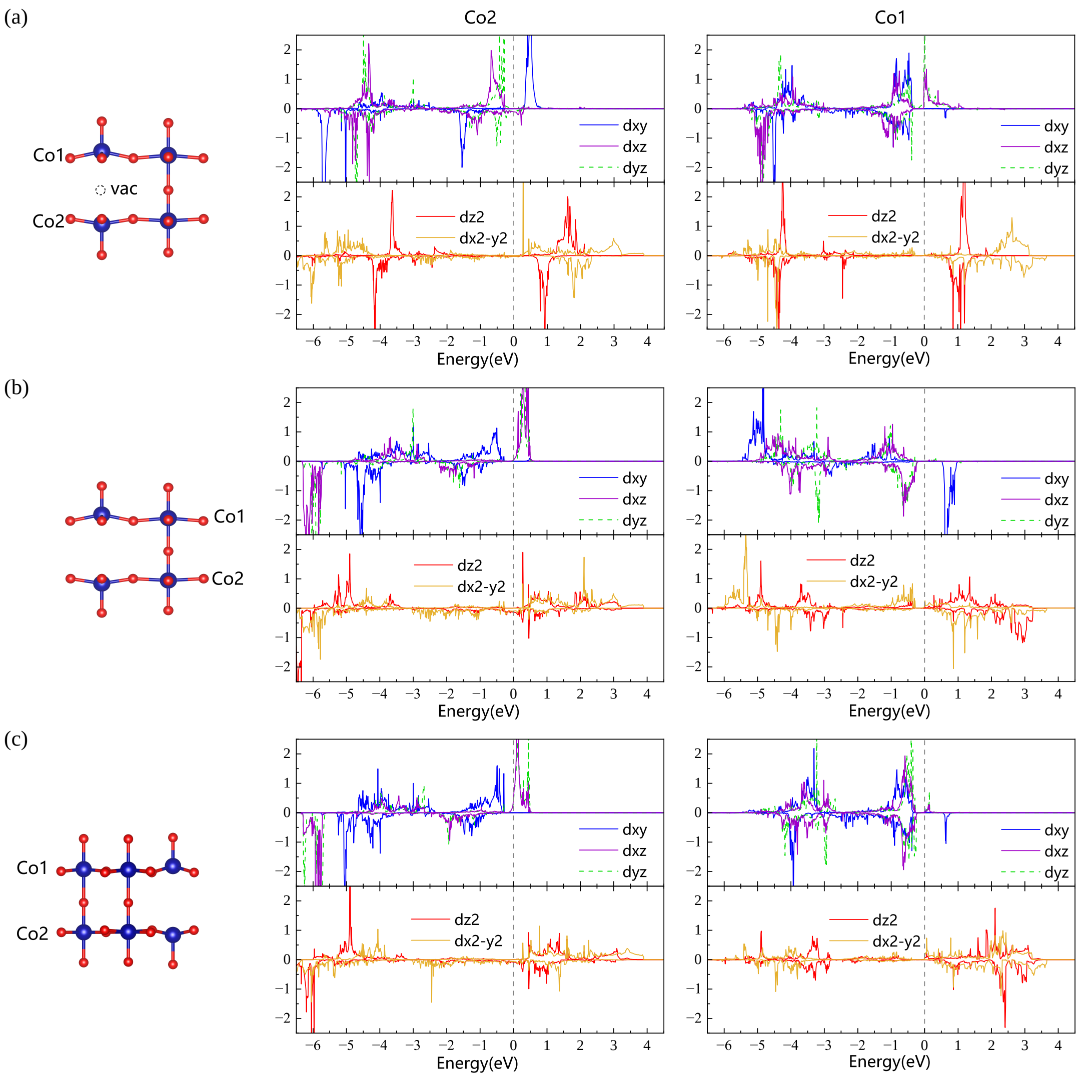


Figure S3. The projected density of states (PDOS) of Co(3*d*) orbitals in the FE phase supercell with an oxygen vaccancy at the apical Oz site. (a) The two Co atoms that have lost their apical-oxygen connections, (b) located near the vacancy, (c) located diagonally opposite the vacancy.
